# Supplementary material for: A Review of Causal Decision Making
Source: arXiv:2502.16156 source file (2025-02-22)
Supplement: Supplementary file 1 [file 11_Appendix.tex]

\section{Appendix}

\begin{table}[tbh]
    \centering
    \begin{tabular}{l|l}
    \hline
    \textbf{Acronym} & \textbf{Meaning}\\
    \hline
        CDM & Causal Decision Making\\
        CSL &  Causal Structure Learning\\
        CEL & Causal Effect Learning\\
        CPL & Causal Policy Learning\\
        OPE & Off-Policy Evaluation\\
        OPO & Off-Policy Optimization\\
        RL  & Reinforcement Learning\\ 
        MDP  & Markov Decision Process\\ 
        POMDP  & Partially Observable Markov Decision Process\\ 
        DTR  & Dynamic Treatment Regime\\ 
        DAG  & Direct Acyclic Graph\\ 
        ATE  & Average Treatment Effect\\ 
        HTE  & Heterogeneous Treatment Effect\\ 
        ATT  & Average Treatment Effect on the Treated \\
        TE  & Total Effect\\ 
        DE  & Direct Effect\\ 
        IE  & Indirect Effect\\ 
        SE  & Spillover Effect\\ 
        SUTVA  & Stable Unit Treatment Value Assumption\\ 
        NUC  & No Unmeasured Confounders\\ 
        OLS  & Ordinary Least Squares\\ 
        MEC  & Markov equivalence class\\ 
        CPDAG  & Completed Partially Directed Acyclic Graph\\  
        SEM  & Structural Equation Model\\  
        LSEM &  Linear Structural Equation Model \\  
        DM  & Direct Method\\  
        IPW  & Inverse Probability Weighting\\  
        DR  & Doubly Robust\\  
        IV  & Instrumental Variable\\  
         DiD  & Difference-in-Difference\\  
        SC  & Synthetic Control\\  
        MBRL & Model-Based Reinforcement Learning\\  
        EG  & Epsilon Greedy\\  
        UCB  & Upper Confidence Bound\\  
        TS  & Thompson Sampling\\  
        MAB  & Multi-Armed Bandit\\  
        CB  & Contextual Bandit\\  
        TD  & Temporal Difference\\  
        SCM  & Structural Causal Models\\  
    \hline
    \end{tabular}
    \caption{Acronyms}
    \label{tab:my_label}
\end{table}
